# Supplementary material for: Unpaired Learning for High Dynamic Range Image Tone Mapping
Source: arXiv:2111.00219 source file (2021-10-30)
Supplement: Supplementary file 1 [file Appendix.tex]

\section*{Appendix A}

The FID measures the distance between the distribution of two image classes by modeling their neural activations using multivariate Gaussians and measuring their Fréchet distance. More specifically, the 2048-dimensional activation vectors produced at the last layer of the Inception-v3 classification network are used. Fitting a Gaussian stably is typically done with using 10,000 samples or more. Since each image produces one sample vector, this is the number of images needed from each class in order to estimate the FID. 

Datasets of HDR images do not offer these numbers of samples and do not permit the use of the FID. To overcome this limitation we consider the pooled activations in the last Inception layer of the Inception Module B. This layer consists of a spatial array of $8 \times 8 $ pixels, each containing an 768-dimensional activation vector. Thus, compared to the original FID where every image provides a single sample vector, switching to this layer results in 64 samples per image. 

We term this modified distance \emph{pixFID} and compare it to the original FID in Figure~\ref{fig:FIDconv}. We used only 1,000 images to evaluate the pixFID in this comparison, next to 50,000 images used to evaluate the FID. The comparison shows the response of these distances to three types of disturbances that were applied to natural images. In case of the Gaussian blur and the additive noise, the pixFID followed the trend of the FID and increased as the disturbance magnitude increased, implying its ability to identify such low-level discrepancies.

In case of a geometric swirl distortion, which does not change the color and shape distribution of small image patches, the pixFID showed an inferior sensitivity to the transformation magnitude. This behaviour is consistent with the fact that activations from a lower level in the network correspond to smaller receptive field and hence to a visual sensitivity to smaller scale features in the image.

\begin{figure}[t]
\centering
\includegraphics[height=3cm]{figs/f.pdf}
  \caption{The response of the FID, red plot, and the pixFID, blue plot, to three types of image disturbances are shown. The FID is computed over 50,000 images whereas the pixFID over 1,000 images.}
  \label{fig:FIDconv}
\end{figure}

Nevertheless, HDR tone-mapping procedures typically does not suffer from geometric or semantic distortions, but from low-level effects such as loss of local contrast, exaggerated details, and edge-related halos.
